# Supplementary material for: On the Nystrom Approximation for Preconditioning in Kernel Machines
Source: arXiv:2312.03311 source file (2024-01-24)
Supplement: Supplementary file 1 [file notation_appendix.tex]

\begin{table}[t]
    \centering
    \begin{tabular}{ll}\toprule
        $n$ & number of samples\\
        $x_i {\in\Real^d},y_i\in\Real$ & training input, label\\
        $K:\Real^d\times\Real^d\rightarrow\Real$ & kernel function\\
        $\mcH_K$ & RKHS space associated with $K$\\
        $\rho$ & input distribution\\
         $\mcT:\Hilbert_K\rightarrow\Hilbert_K$ & $\int_{\Real^d} K(x,\cdot)\otimes K(x,\cdot)\rho(\dif x)$\\
        $\mcK:\Hilbert_K\rightarrow\Hilbert_K$ &
        $\frac1n\sum_{i=0}^nK(x_i,\cdot)\otimes K(x_i,\cdot)$\\
        $\kappa(\cdot)$ & condition number ({\sf CN}) of $\cdot$\\
        $\beta(K)$ & $\lmax_x K(x,x)$\\
        \midrule
        $\kappa_1$ & $\kappa(\mcK)$ ({\sf CN w/o} preconditioning)\\
        $\mcP_q$ & preconditioner with level $q\in\Natural$\\
        $\kappa_q$ & $\kappa(\mcP_q\circ\mcK)$ ({\sf CN w/} preconditioning)\\
        \midrule
        $s$ & number of Nystr\"om samples\\
        $\mcK':\Hilbert_K\rightarrow\Hilbert_K$&  $\frac1s\sum_{i=0}^sK(x_{t_i},\cdot)\otimes K(x_{t_i},\cdot)$\\
        $\mcP_{s,q}$& approximated  preconditioner\\
        $\kappa_{s,q}$ & ({\sf CN w/} approx.\ preconditioning)\\
        &$\kappa(\sqrtop{\mcP_{s,q}}
        \circ\mcK\circ\sqrtop{\mcP_{s,q}})$\\
        \bottomrule
    \end{tabular}
    \caption{Notation}
    \label{tab:notation_appendix}
\end{table}
